# Supplementary material for: Using Large Language Models to Develop Requirements Elicitation Skills
Source: arXiv:2503.07800 source file (2025-04-09)
Supplement: Supplementary file 1 [file exercise-metrics.tex]

\begin{tabular}{llrr}
\toprule
 & Group & Control Group & Experimental Group \\
Metric & Statistic &  &  \\
\midrule
\multirow[t]{8}{*}{Duration}
 & 25\% & 0.76 & 0.72 \\
 & 50\% & 0.84 & 0.81 \\
 & 75\% & 0.93 & 0.99 \\
 & count & 59.00 & 61.00 \\
 & max & 1.34 & 1.39 \\
 & mean & 0.86 & 0.85 \\
 & min & 0.38 & 0.42 \\
 & std & 0.19 & 0.23 \\
\cline{1-4}
\multirow[t]{8}{*}{Mean time between Interactions(secs)}
 & 25\% & - & 73.07 \\
 & 50\% & - & 91.71 \\
 & 75\% & - & 128.36 \\
 & count & 0.00 & 61.00 \\
 & max & - & 196.38 \\
 & mean & - & 103.48 \\
 & min & - & 45.83 \\
 & std & - & 36.84 \\
\cline{1-4}
\multirow[t]{8}{*}{Mean IA response length (characters)}
 & 25\% & - & 190.76 \\
 & 50\% & - & 236.67 \\
 & 75\% & - & 279.41 \\
 & count & - & 61.00 \\
 & max & - & 538.19 \\
 & mean & - & 236.24 \\
 & min & - & 90.78 \\
 & std & - & 78.35 \\
\cline{1-4}
\multirow[t]{8}{*}{Mean participants question length (chars)}
 & 25\% & - & 56.87 \\
 & 50\% & - & 72.50 \\
 & 75\% & - & 85.37 \\
 & count & 0.00 & 61.00 \\
 & max & - & 178.65 \\
 & mean & - & 74.44 \\
 & min & - & 30.30 \\
 & std & - & 26.26 \\
\cline{1-4}
\multirow[t]{8}{*}{nAttributes in participants solutions }
 & 25\% & 22.00 & 12.00 \\
 & 50\% & 27.00 & 14.00 \\
 & 75\% & 33.00 & 17.00 \\
 & count & 59.00 & 60.00 \\
 & max & 62.00 & 35.00 \\
 & mean & 28.32 & 15.30 \\
 & min & 12.00 & 6.00 \\
 & std & 8.83 & 4.97 \\
\cline{1-4}
\multirow[t]{8}{*}{nClasses  in participants solutions}
 & 25\% & 9.00 & 7.00 \\
 & 50\% & 10.00 & 8.00 \\
 & 75\% & 12.00 & 9.00 \\
 & count & 59.00 & 60.00 \\
 & max & 18.00 & 12.00 \\
 & mean & 10.61 & 7.68 \\
 & min & 6.00 & 4.00 \\
 & std & 2.67 & 1.57 \\
\cline{1-4}
\multirow[t]{8}{*}{score (as computed by chat gpt) \textbf{Should we omit this?}} 
 & 25\% & 5.00 & 3.00 \\
 & 50\% & 5.50 & 5.00 \\
 & 75\% & 6.00 & 5.00 \\
 & count & 58.00 & 61.00 \\
 & max & 8.00 & 7.00 \\
 & mean & 5.36 & 4.36 \\
 & min & 3.00 & 0.00 \\
 & std & 1.04 & 1.32 \\
\cline{1-4}
\bottomrule
\end{tabular}
